# Supplementary material for: Deep density ratio estimation for change point detection
Source: arXiv:1905.09876 source file (2019-05-23)
Supplement: Supplementary file 1 [file cpd_manuscript_supp.pdf]

## Appendix

### Density Ratio Based CPD

These methods perform change point detection by first learning an approximation to the density ratio function. During inference, the learned function is applied to the input signal and the change point is determined using a thresholding function.

**KLIEP** The Kullback-Leibler Importance Estimation Procedure is a density ratio estimation method that uses kernel functions, typically gaussian kernels, to approximate the density ratio. Specifically, the density ratio is approximated by a weighted combination of kernels:

$$f(x; \theta) = \sum_{l=1}^b \theta_l \phi(x, x_l)$$

The parameters  $\theta$  are learned by solving the convex optimization problem given in Equation 1 which minimizes the KL-divergence between the reference distribution and the approximation Sugiyama et al. [2008].

**rULSIF** Similar to KLIEP, Relative Unconstrained Least Squares Importance Fitting uses kernels to approximate the density ratio, however a different optimization problem is solved to learn the parameters. The objective function is derived using the squared loss and is written as:

$$\frac{1}{2n_r} \sum_{x \in \mathcal{X}} f(x; \theta)^2 - \frac{1}{n_e} \sum_{x \in \mathcal{X}} f(x; \theta)$$

For a complete description, see Liu et al. [2013].<sup>2</sup>

**DDRE** Deep Density Ration Estimation uses a deep feedforward network as a function approximator to the density ratio. We compare three objective functions for training the deep feedforward network:

- DDRE-LSIF: trained using the LSIF objective (Equation 2) [Nam and Sugiyama, 2015].
- DDRE-DSKL: trained using the DSKL objective (Equation 3).
- DDRE-BARR: trained using the BARR objective (Equation 4).

For each of these objective functions, we use a five layer rectified linear unit (ReLU) network Nair and Hinton [2010]. The first four layers are 500 units wide each. The output layer consists of one unit with a ReLU activation function as the density ratio function is nonnegative. L2 regularization with  $\lambda = 0.01$  was applied to each layer as well as Dropout Agarwal et al. [2011] with keep probability 0.5. The network was trained using the ADAM Kingma and Ba [2014] optimizer and minibatch gradient descent. Training was continued until the objective stopped decreasing, typically 50-100 epochs. This network structure was fixed in all of our experiments to ensure fair comparison between the objective functions. Our implementation was written using Tensorflow [Abadi et al., 2016].

**DCDRE** We also experimented with a convolutional neural network using the DSKL objective function. We borrowed the architecture of this network from the CNN trained on EEG data in Khan et al. [2018] except for the last layer. The network consists of six convolutional and max-pooling layers followed by three fully connected layers ending in a single unit. The convolutional and pooling structure of the network is shown in Table 1. The network contains ReLU activation functions at every layer as well as L2 regularization ( $\lambda = 0.01$ ) and Dropout ( $p = 0.25$ ). The ADAM optimizer and minibatch gradient descent ( $bS = 100$ ) were used to train the network.

### Window Based CPD

These methods perform change point detection using two sliding windows along the signal. A discrepancy measure is computed at each time point using a cost function. Peaks in the discrepancy measure are considered change points. Each of the following methods defines a different cost function for computing the discrepancy. Following is a short description of each, for details see [Truong et al., 2018].<sup>3</sup>

<sup>2</sup>We used the Matlab code for KLIEP and rULSIF provided by the authors at <http://www.ms.k.u-tokyo.ac.jp/software.html>

<sup>3</sup>We used the python code provided by the authors in our experiments <https://github.com/deepcharles/ruptures>

Table 1: Convolutional network architecture for EEG data Khan et al. [2018].

| Type        | Units | Size | Stride |
|-------------|-------|------|--------|
| Conv2D      | 60    | 3x3  | 1      |
| Pool2D      |       | 2x2  | 1      |
| Conv2D      | 50    | 3x3  | 1      |
| Conv2D      | 40    | 3x3  | 1      |
| Pool2D      |       | 2x2  | 1      |
| Conv2D      | 20    | 3x3  | 1      |
| Pool2D      |       | 2x2  | 1      |
| Conv2D      | 10    | 2x2  | 1      |
| Conv2D      | 5     | 2x2  | 1      |
| Fully Conn. | 250   |      |        |
| Fully Conn. | 100   |      |        |
| Output      | 1     |      |        |

405 **KCPD** Kernel Change Point Detection algorithms use a kernel function that maps the signal onto a reproducing  
406 kernel Hilbert space to measure the cost. A typical choice of kernel function is the Gaussian kernel.

407 **ARCPD** Auto Regressive Change Point Detection uses deviations or residuals from a linear auto regressive  
408 model to model the cost between adjacent windows.

409 **L2CPD** L2 Change Point Detection uses the Euclidean distance to measure the cost.

410 **L1CPD** L1 Change Point Detection uses the L1 distance as the cost function.

Table 2: Mount Sinai Hospital EEG dataset statistics.

|                |        |
|----------------|--------|
| # Recordings   | 121    |
| Average Length | 1.55h  |
| # Channels     | 22     |
| # Features     | 396    |
| Window Length  | 5s     |
| # Windows      | 143803 |
